# Supplementary material for: Escalation Prediction using Feature Engineering: Addressing Support Ticket Escalations within IBM's Ecosystem
Source: arXiv:2010.06390 source file (2020-10-12)
Supplement: Supplementary file 3 [file chapter_app_c.tex]

\startappendix{Publications}
\label{appendix:c}

\includepdf[pages=-,scale=.9,pagecommand={}]{re17_full_paper.pdf}

\includepdf[pages=-,scale=.9,pagecommand={}]{re17_tool_paper.pdf}
